# Supplementary material for: Regaining Trust: Impact of Transparent User Interface Design on Acceptance of Camera-Based In-Car Health Monitoring Systems
Source: arXiv:2408.15177 source file (2024-08-27)
Supplement: Supplementary file 1 [file appendix.tex]

\newpage
    \section{Appendix}

\begin{figure*}[ht]
      \centering
    \includegraphics[width=0.49\textwidth]{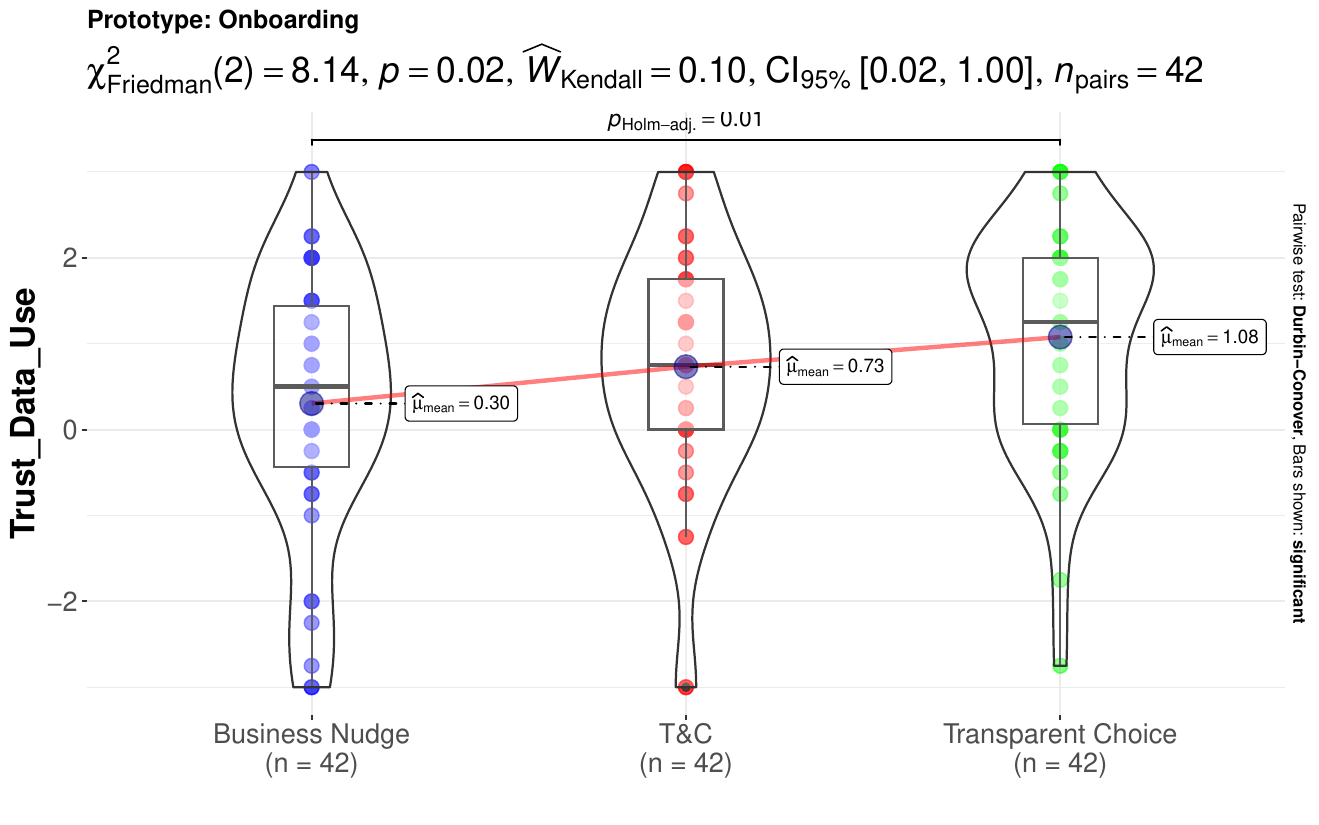}
    \includegraphics[width=0.49\textwidth]{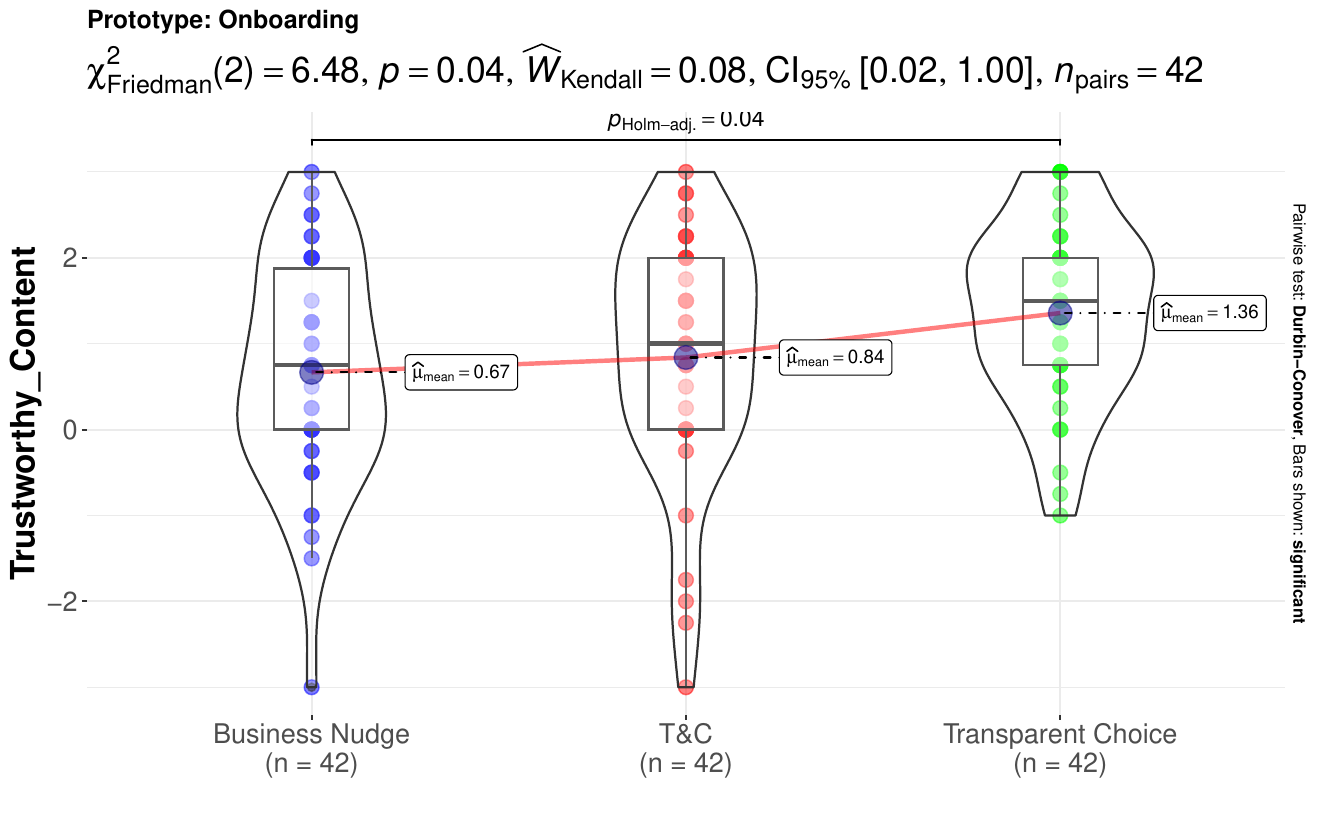}
\captionsetup{width=0.6\textwidth}   
\caption{Trust and Trustworthiness of the Onboarding Prototypes [H3].}
      \Description{Trust and Trustworthiness of the Onboarding Prototypes [H3].}
    \label{fig:OnboardingTrust}
\end{figure*}

\begin{figure*}[ht]
      \centering
  \includegraphics[width=0.49\textwidth]{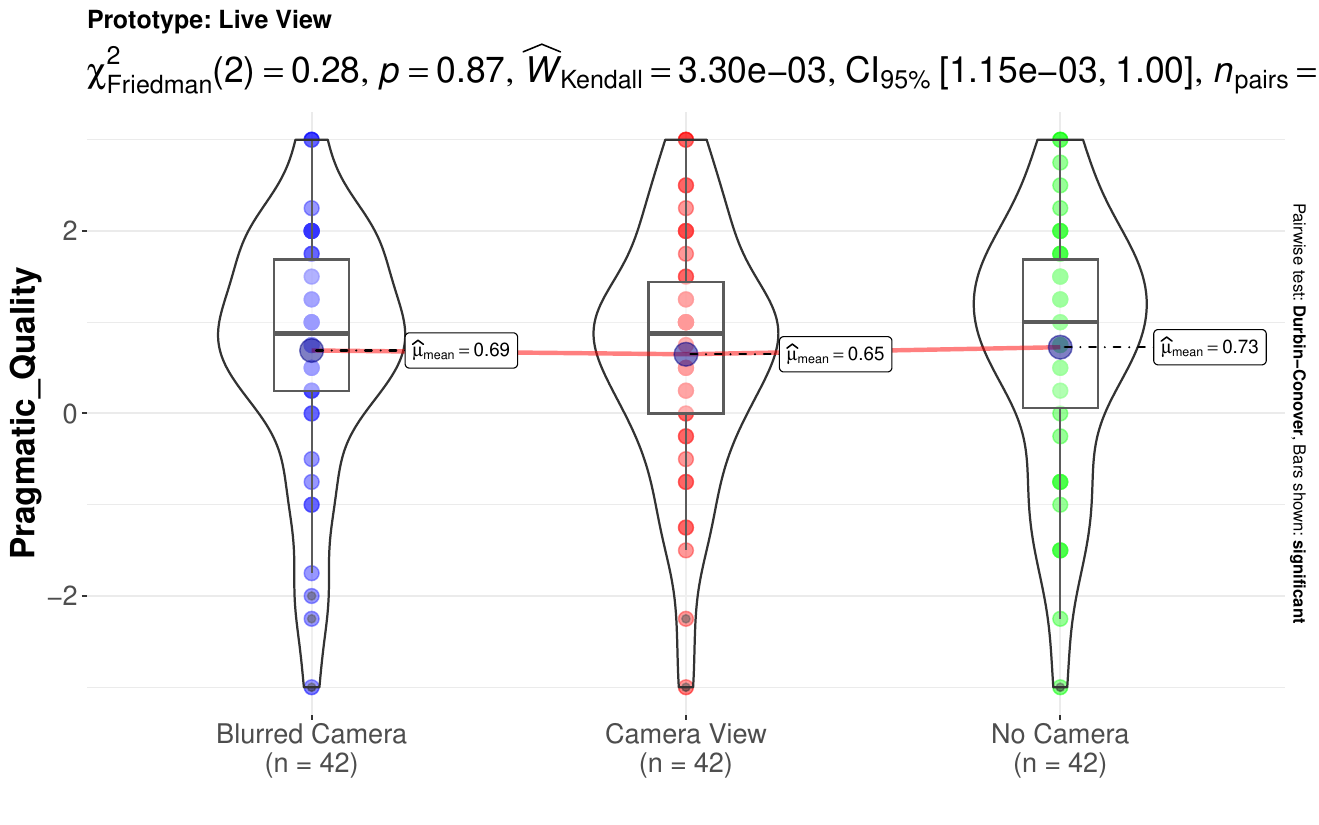}
    \includegraphics[width=0.49\textwidth]{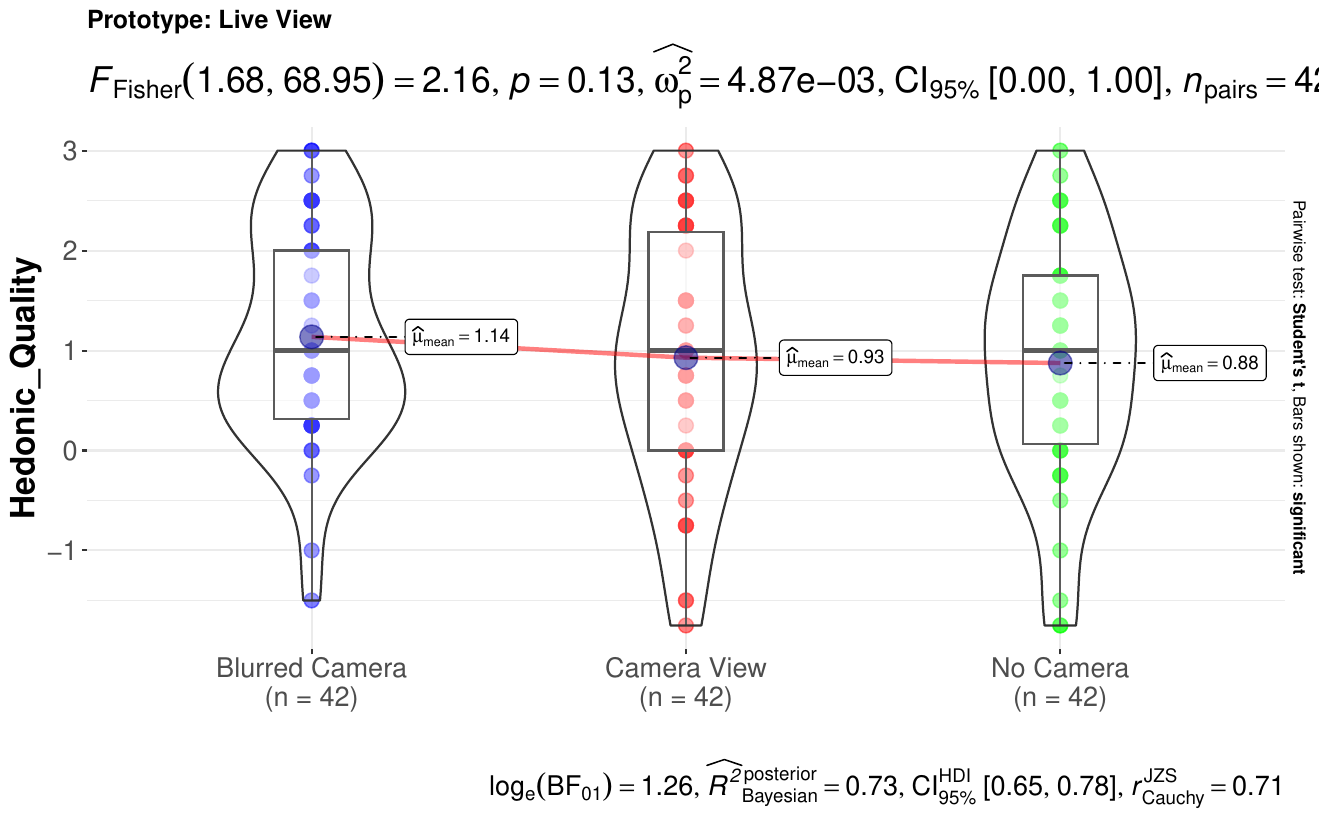}
\captionsetup{width=0.6\textwidth}   
\caption{User Experience of the Live View Prototypes as measured by Pragmatic [H4] and Hedonic Quality [H5].}
      \Description{User Experience of the Live View Prototypes as measured by Pragmatic [H4] and Hedonic Quality [H5].}
    \label{fig:LiveViewUX}
\end{figure*}

\begin{figure*}[ht]
      \centering
    \includegraphics[width=0.49\textwidth]{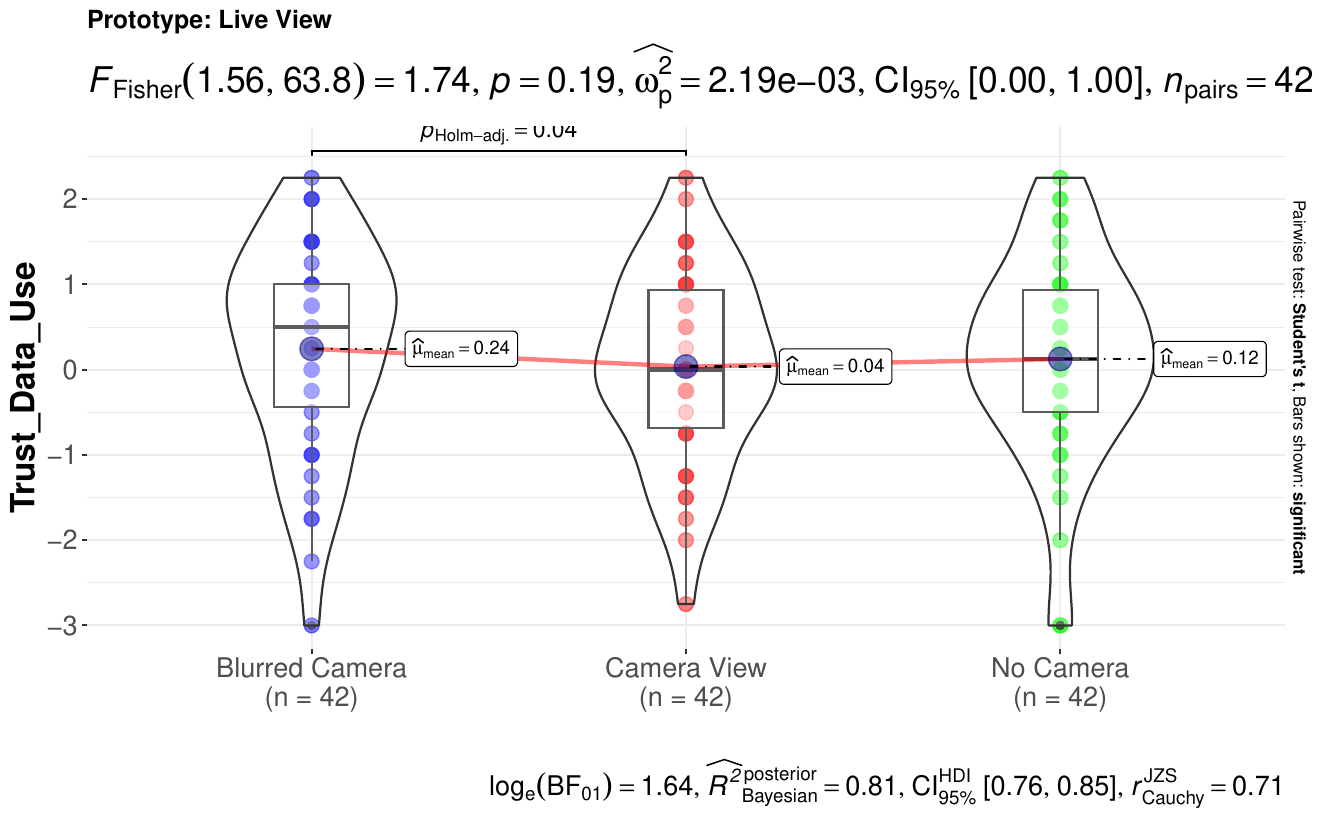}
    \includegraphics[width=0.49\textwidth]{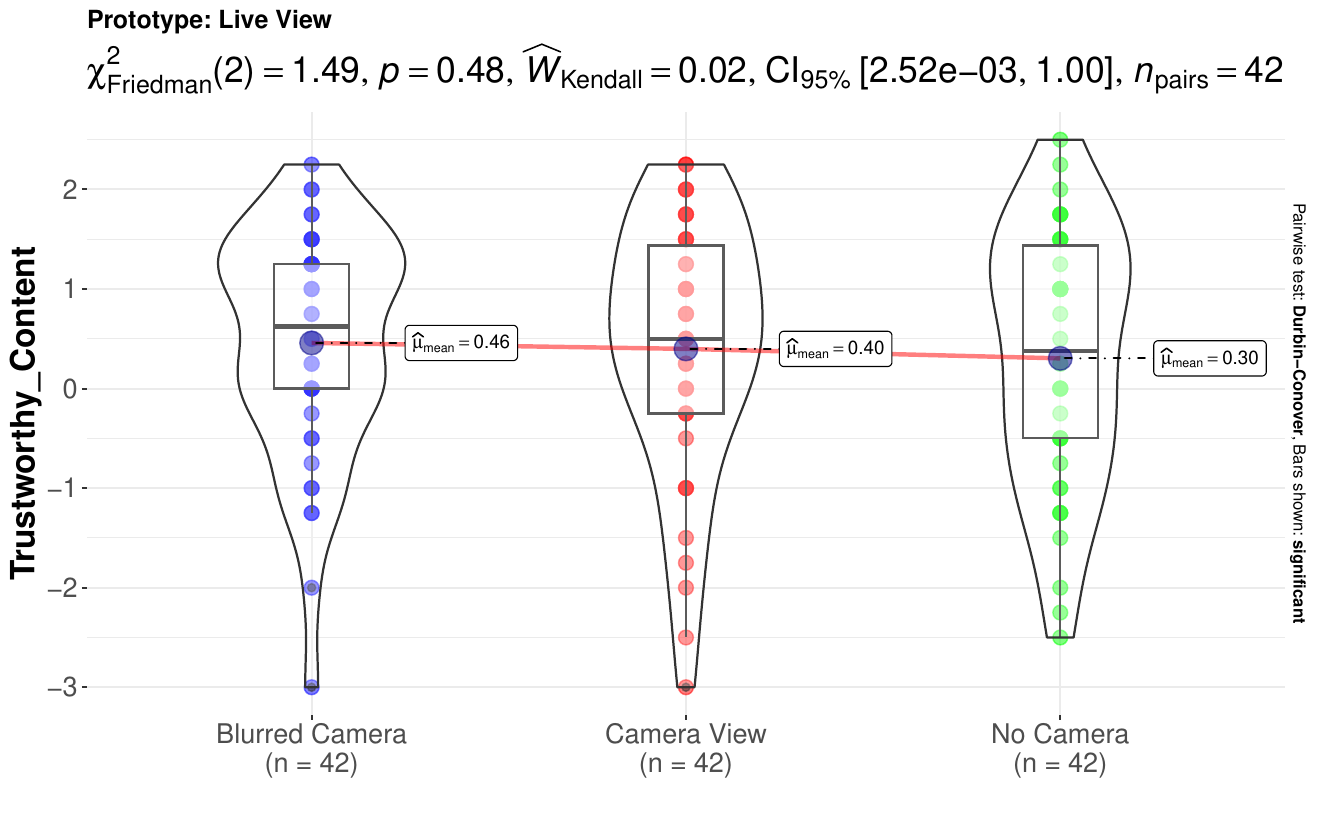}
\captionsetup{width=0.6\textwidth}   
\caption{Trust and Trustworthiness of the Live View Prototypes as measured by Hedonic and Pragmatic Quality [H6].}
      \Description{Trust and Trustworthiness of the Live View Prototypes [H6].}
    \label{fig:LiveViewTrust}
\end{figure*}

\begin{figure*}[t]
      \centering
    \includegraphics[width=0.49\textwidth]{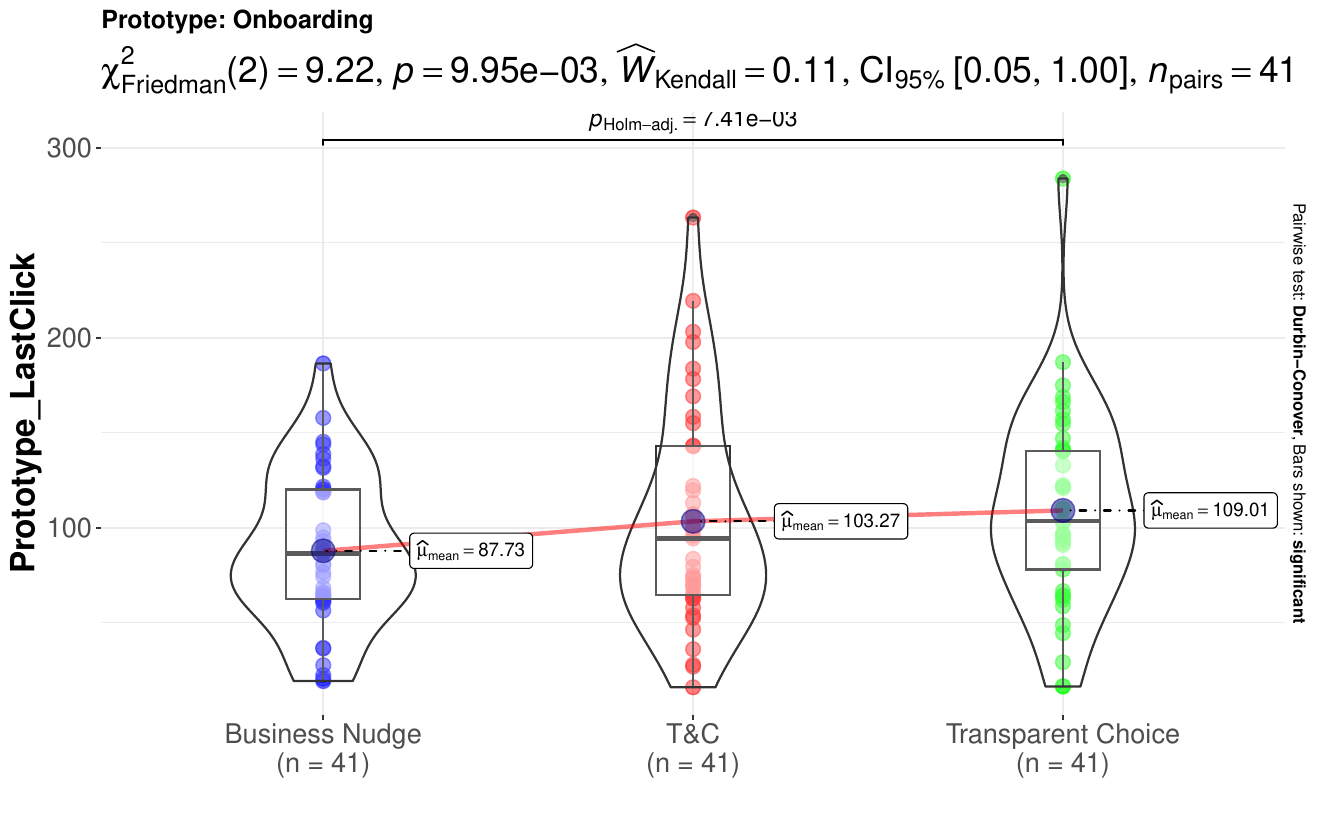}
\captionsetup{width=0.6\textwidth}   
\caption{Time spent evaluating the Onboarding prototype [H7].}
      \Description{Time spent evaluating the Onboarding prototype [H7].}
    \label{fig:LastClicks}
\end{figure*}

\begin{figure*}[t]
      \centering
       \includegraphics[trim=34cm 7cm 79cm 25cm, clip=true, width=1.0\textwidth]{Figures/Mock-up.pdf}
\captionsetup{width=1.0\textwidth}   
\caption{Zoomed-in view of the Freeform board for designing the Mockups. These wireframes are similar to the final implemented prototype.}
      \Description{Zoomed-in view of the Freeform board for designing the Mockups. These wireframes are similar to the final implemented prototype.}
    \label{fig:Mockup}
\end{figure*}

\begin{table}[ht]
\centering
\small
\begin{tabular}{|l|p{6.2cm}|c|c|c|}
\hline
\textbf{Scale} & \textbf{Items} & \textbf{Mean} & \textbf{SD} & \textbf{Cronbach's $\alpha$} \\ 
\hline
Pragmatic Quality & \makecell[l]{I think the technology and user interface is:\\ - obstructive:supportive \\ - complicated:easy \\- inefficient:efficient \\ - confusing:clear} & 1.3 & 1.2 & 0.875 \\
\hline
Hedonic Quality & \makecell[l]{I think the technology and user interface is: \\ - boring:exciting \\ - not interesting:interesting \\ - conventional:inventive \\ - usual:leading edge} & 1.29 & 1.3 & 0.932 \\
\hline

Trustworthy Content & \makecell[l]{In my opinion, the information and data \\provided by the product are:\\ - useless:useful \\ - implausible:plausible \\- untrustworthy:trustworthy \\- inaccurate:accurate} & 0.87 & 1.09 & 0.801 \\
\hline
Trust Data Use & \makecell[l]{Regarding the use of my personal information \\and data, the product is:\\ - insecure:secure \\ - untrustworthy:trustworthy \\- unreliable:reliable \\ - non-transparent:transparent} & 0.53 & 1.25 & 0.871 \\
\hline
Creepy & \makecell[l]{Strongly disagree:strongly agree:\\- I find this technology creepy. \\- This technology makes me feel uncomfortable. \\- The way this technology uses (personal) \\information is unsettling.} & -1.3 & 1.66 & 0.965 \\ 
\hline

\end{tabular}
\caption{Tect of suibcale items and scale reliability statistics (N=12).}
   \label{tab:scalereliability}
\end{table}
